# Supplementary material for: Further Understanding of a Local Gaussian Process Approximation: Characterising Convergence in the Finite Regime
Source: arXiv:2404.06200 source file (2024-04-09)
Supplement: Supplementary file 1 [file au_convergence.tex]

\section{Almost Uniform Convergence}

Suppose we know that the predictions are insensitive, then:
\begin{lemma}[Prediction insensitivity]
\label{lem:pred_insensitivity_TV}
    Let \(\TV(p(f^*\given \yv,\thv_1),p(f^*\given\yv,\thv_2))\leq\varepsilon\) for all \(\thv_1,\thv_2 \in \Theta \backslash T\) where \(\Theta \subseteq \support(\Pi_n)\) and \(\Pi_n(T)=0\). Then,
    \begin{equation*}
        \TV(p(f^*\given\yv),p(f^*\given\yv,\thv)) \leq \varepsilon
    \end{equation*}
    a.e. w.r.t \(\Pi_n(\thv)\).
\end{lemma}
\begin{proof}
    For brevity set \(q_i=p(f^*\given\yv,\thv_i)\) for some choice of \(\thv_i \in \Theta \backslash T\), \(q(\thv)=p(f^*\given\yv,\thv)\) and \(p=p(f^*\given\yv)\) and the posterior density is \(\pi_n(\thv)\).
    \eq{
    \TV(p,q_i) &= \int\abs{\int q(\thv)\pi_n(\thv)d\thv - q_i}df^* \\
    &= \int\abs{\int(q(\thv)-q_i)\pi_n(\thv)d\thv}df^* \\
    &\leq \int\int\abs{q(\thv)-q_i}\pi_n(\thv)d\thv df^* \\
    &= \int\pi_n(\thv)\int\abs{q(\thv)-q_i}df^* d\thv \\
    &=\int \TV(q(\thv),q_i)\pi_n(\thv)d\thv \\
    &= \E_{\thv\sim\Pi_n}\left[\TV(q(\thv),q_i)\right] \\
    &\leq \varepsilon
}
\end{proof}

\begin{remark}
    \cref{lem:pred_insensitivity_TV} can be modified to state that if \(\Ey{\TV(q_1,q_2)}<\varepsilon\) then \(\Ey{\TV(p,q_{\thv})}<\varepsilon\), since we can exchange the expectations over \(\yrv\) and \(\thv\) as they are both finite. The proof follows exactly the same as \cref{lem:pred_insensitivity_TV} but with the final line swapping the order of expectation.
\end{remark}

\begin{lemma}[\(\varepsilon\)-insensitivity assumption]
\label{lem:ass_insensitivity}
    Given predictive Gaussian process distributions \(q_i=p(f^*\given \yv,\thv_i)\) with predicted mean and variance \((\mu_i,\sigma_i^2)\) such that \(\Ey{\abs{\mu_i-y^*}}^2=\sigma_i^2\) and \(\abs{\sigma_1^2-\sigma_2^2} < \varepsilon\) then
    \[\Ey{\KL(q_1,q_2)} < \frac{3\varepsilon}{\sigma_2^2}\] and 
    \[\Ey{\TV(q_1,q_2)} < \sqrt{\frac{3\varepsilon}{2\sigma_2^2}}\]
    under the sufficient conditions that \(\abs{v_1-v_2}<\varepsilon\), \(\abs{v-v_2}<\varepsilon\) and \(\abs{v-v_1}<\varepsilon\) where \(\sigma_i^2 = v_i - \kappa_i\) and \(\kappa_i=\kstar^T_iK_i^{-1}\kstar_i\).
\end{lemma}
\begin{proof}
    WLOG let \(\sigma_1>\sigma_2>0\) so that \(0<\sigma_1^2-\sigma_2^2<\varepsilon\). Then,
    \eq{
        \KL(q_1,q_2) &< \frac{\varepsilon}{2\sigma_2^2} + \frac{(\mu_1-\mu_2)^2}{2\sigma_2^2} \\
        \Ey{(\mu_1-\mu_2)^2} &= \E_{\mathbf{y}} \big\{(\mu_1-y^*)^2 + (\mu_2-y^*)^2 \\
        &-2(\mu_1-y^*)(\mu_2-y^*)\big\} \\
        &= \sigma_1^2 + \sigma_2^2 \\
        &- 2\Ey{(\mu_1-y^*)(\mu_2-y^*)} \\
        \Ey{(\mu_1-y^*)(\mu_2-y^*)}&= v - \kappa_1 - \kappa_2 + \Ey{\mu_1\mu_2}
    }
    Now the key term is \(\Ey{\mu_1\mu_2}\) which can be shown in the limit to attain \(\sigma_f^2+m^{-1}\sigma_\xi^2 -m^{-1}\sigma_f^2\left(\frac{\sigma_{1,\xi}^2}{\sigma_{1,f}^2} + \frac{\sigma_{2,\xi}^2}{\sigma_{2,f}^2}\right)\).
    If we can further assume that \(\Ey{\mu_1\mu_2}=\kstar_1^TK_1^{-1}KK_2^{-1}\kstar_2 \geq \kappa_1-\varepsilon\) (which we believe to be a plausible assumption, satisfied if e.g. the \emph{external} parameters exactly match) then \(\Ey{(\mu_1-y^*)(\mu_2-y^*)} \geq v-\kappa_1-\kappa_2+\kappa_1-\varepsilon\) and
    \eq{
        \Ey{(\mu_1-\mu_2)^2} &\leq \sigma_1^2 + \sigma_2^2 - 2(v-v_2)-2\sigma_2^2+2\varepsilon \\
        &< 3\varepsilon -2(v-v_2) \\
        &< 5\varepsilon \qquad (\textrm{by assumption})
    } and
    \eq{
        \Ey{\KL(q_1,q_2)} &< \frac{\varepsilon}{2\sigma_2^2} + \frac{5\varepsilon}{2\sigma_2^2} = \frac{3\varepsilon}{\sigma_2^2}
    }
    Then Pinsker's inequality combined with Jensen's inequality gives
\eq{
    \Ey{\TV(q_1,q_2)} &< \sqrt{\frac{3\Ey{\KL(q_1,q_2)}}{2}} < \sqrt{\frac{3\varepsilon}{2\sigma_2^2}}
}
\end{proof}
\todo{tighten up, check all inequalities and all assumptions needed. Check what happens if we switched ordering (should be arbitrary)}

\begin{remark}
    Using Markov's inequality, we can then convert this to say that with probability at least \(1-\sqrt{\frac{3}{2}}\frac{\varepsilon}{\sigma_2}\), \(\TV(q_1,q_2) \leq \varepsilon\), if \(\abs{\sigma_1^2-\sigma_2^2}\leq \varepsilon^4\). etc
\end{remark}

\begin{remark}
    \cref{lem:ass_insensitivity} gives conditions under which we can bound the expected value of the KL (and TV) between two predictive distributions differing in their choice of hyperparameters such that their MSEs are close. These conditions effectively add additional restrictions on the kernelscale and noise variance parameters for this to hold. The implication of this is that, when combined with \cref{lem:pred_insensitivity_TV}, we can say that for (almost) uniform convergence to occur over the lengthscale (or similar internal kernel parameters) the external parameters must be close to optimal. Fortunately, this situation is exactly that which the recalibration step seeks to address.
\end{remark}
