# Supplementary material for: Further Understanding of a Local Gaussian Process Approximation: Characterising Convergence in the Finite Regime
Source: arXiv:2404.06200 source file (2024-04-09)
Supplement: Supplementary file 2 [file old_full_nn_proof.tex]

\robertcomment{Tomasz: Sorry we should have explained when we all last met and saved you the trouble of checking the long proof below which Ant is due to remove from the paper : After a detailed look my earlier checking revealed (a) an error in Ant's proof  and (b) (partly because the error meant pulling back some extra generality Ant was hoping to add) it is possible to replace this entire proof with an extremely short one (now summarised in the main text}.
\antcomment{I didn't recall there being an error? Just that we were hoping to reduce it - but haven't yet, so I'm appreciative of Tomasz having a look}
\robertcomment{The error I meant was present when the proof aimed to cover the generality of kernelswhose assocoiated metrics  were not bounded everywhere by powers of delta (e.g. periodic kernels). I think that erroneous part has probably now been removed. My point was that aiming for that generality is probably what had led to you pursuing this extensive proof which, once you use the everywhere-applicable  simple 'power of delta' upper bounds to the kernel metric, is no longer needed} 
\newline\newline
\robertcomment{I also very much appreciate Tomasz' perspectives on the presentational aspects of the proof, but priority for remaining time is to check the other parts of the paper on the basis that this part is to be removed }

\subsubsection{Proof of \cref{lem:eps_i}}
\label{proof:eps_i}
    The strategy we adopt to prove this result can be broken down into the steps enumerated below, for which we need the following definitions:
    \eq{
        S_{\zrv,r} &:= \left\{\xrv \in \mc{X} :\norm{\xrv-\zrv} < r\right\},\, \zrv\in\mc{X}, r>0
    }
        and the \(\eps\)-covering number \(N(A,\norm{\cdot},\eps)\) over a subset \(A\) of a metric space \((A,\norm{\cdot})\) that satisfies
    \eq{
        A \subseteq \bigcup_{\xv\in C}S_{\xv,\eps}
    }
    for some \(C\subseteq M\).
    \begin{enumerate}
        \item Divide the input space into a series of concentric sets,
        \item Find an \(\eps\)-covering number for each of these sets,
        \item Use the covering number to bound the expected value over each set from above,
        \item Segment the training data such that the nearest neighbour to the test point from each segment is equally close to the test point in expectation (over \(X\)). \tomcomment{I didn't get this at first. Only after reading the proof, I think I know what you mean here, but this point 4 somehow only made me more confused. Maybe try to rephrase it somehow?}
    \end{enumerate}
    
    We evaluate \(\E\eps_i\) using Theorem 6.2 from \cite{Gyorfi2010} and Lemma 1 from \cite{Kohler2006}. Before we can make the final argument, we first need some preliminary results. First, we partition the space into a series of nested sets centred at the origin, \((S_{0,j})_{j=1}^\infty\) so that 
    
    \eq{
        \E_{\xrv} & \big\{\rho^2(\xrv_{(1,n)}(\xrv),\xrv)\big\}  \\
        &= \sum_{j=1}^\infty \E_{\xrv}\left\{\rho^2(\xrv_{(1,n)}(\xrv),\xrv)\1{\xrv\in S_{0,j}\backslash S_{0,j-1}}\right\} \\
        &= \sum_{j=1}^\infty \int_0^\infty\Pr\left\{\rho^2(\xrv_{(1)},\xrv) > \varepsilon, {\xrv\in S_{0,j}\backslash S_{0,j-1}}\right\}d\varepsilon\\
        &\leq \sum_{j=1}^\infty \int_0^\infty\min\bigg\{\mu(S_{0,j}\backslash S_{0,j-1}), \\
        &\qquad\qquad \frac{1}{en}N(S_{0,j}\backslash S_{0,j-1},\norm{\cdot},L'^{-\frac{1}{p}}(\varepsilon-B)^\frac{1}{p})\bigg\}.
        % &\leq \sum_{j=1}^\infty \int_0^1\min\left\{\mu(S_{0,j}\backslash S_{0,j-1}), \frac{c}{en}\frac{j^{d-1}}{\varepsilon^{d/2}}\right\}
    }
    \tomcomment{There is a logical jump in deriving the inequality. Needs to be explained. Also, what is N?}
    
    where we use the integrated tail probability expectation formula whose origins can be found in many statistical texts (e.g. \cite{lo_demystifying_2019}) and the final inequality and associated notation are explained immediately below. Recall the constants \(L,B\) are defined by \ref{ass:kernel_dist} and let \(L'=Ll^{-p}\).

    \tomcomment{State the integrated tail probability expectation formula separately.}
    
    To make progress we bound the inner probability using a covering number:

    \tomcomment{Again, the formulas below use notation that has not been explained before. What is a covering number? What is A? I can see that it is somewhat explained after the formulas, but not in a sufficient way.}
    
    \eq{
        % \Pr\left\{\rho(\xrv_{(1,n)}(\xrv),\xrv)>\varepsilon, X \in A\right\} &\leq \Pr\left\{\norm{\xrv_{(1,n)}-\xrv} > \left(\frac{\varepsilon}{L}\right)^\frac{1}{p}, X \in A\right\} \qquad \textrm{(by \ref{ass:kernel_dist})}\\
        \Pr\{ & \rho^2(\xrv_{(1,n)}(\xrv),\xrv)>\varepsilon, \xrv \in A\} \\
        &\leq \Pr{\Delta_1^{\xrv} > L'^{-\frac{1}{p}}(\varepsilon-B)^\frac{1}{p}, \xrv \in A} \quad \textrm{\ref{ass:kernel_dist}}\\
        &= \int_A \Pr{\Delta_1^{\xv} > \varepsilon'}\mu(d\xv) \\
        &= \int_A(1-\mu(S_{\xv,\varepsilon'}))^n\mu(d\xv)\\
        &\leq \sum_{l=1}^{N(\varepsilon')}\int_{S^l}(1-\mu(S_{\xv,\varepsilon'}))^n\mu(d\xv)\\
        &\leq \sum_{l=1}^{N(\varepsilon')}\int_{S^l}(1-\mu(S^l))^n\mu(d\xv)\\
        &=\sum_{l=1}^{N(\varepsilon')}\mu(S^l)(1-\mu(S^l))^n \\
        &\leq \sum_{l=1}^{N(\varepsilon')}\max_r r(1-r)^n \\
        &\leq \sum_{l=1}^{N(\varepsilon')}\max_r r\e^{-nr} \\
        & = \frac{N(\varepsilon')}{en}
    }
    \tomcomment{Now this is a very long sequence of equations and inequalities with no extra explanation in between. Have a look at the proof of Lemma 6.4 in Gyorfi et al and and see how clearly they explain a similar reasoning sequence. Try to mimic that here.}

    where \(\varepsilon' = L'^{-\frac{1}{p}}(\varepsilon-B)^\frac{1}{p}\) and \(S^1,S^2,\dots,S^{N(r)}\) are a sequence of balls of radius \(r/2\) that cover the set \(A\).

    \tomcomment{Explain this concept of covering A with balls a bit more. Again, for comparison look how Gyorfi et al and Kohler et al. formulate their proofs.}
    
    Now when the set is \(A=A_j=S_{0,j}\backslash S_{0,j-1}\) we have that \(\diam(A)=2j\) and \(N(A,\rho_E,\varepsilon)\leq c\frac{j^{d-1}}{\varepsilon^d}\), since \(\vol(S_{0,j})\leq c_j j^d\), \(\vol(S_{0,j-1})\leq c_{j-1}(j-1)^d = c_{j-1}j^d(1-d/j + \bigO{j^{-2}})\) and hence \(\vol(S_{0,j})-\vol(S_{0,j-1}) \leq (c_j-c_{j-1})j^d + c_{j-1}dj^{d-1} - \bigO{j^{d-2}}\). As the constant \(c_j\) depends only on the dimension, \(c_j=c_{j-1}\,\forall j \in \mathbb{N}\) we have \(\vol(S_{0,j}\backslash S_{0,j-1})\leq c j^{d-1}\). \tomcomment{Is vol just the volume of d-dim sphere? A simple short comment would clarify this.}

    \tomcomment{See my previous four remarks. They way you present this proof now makes the reasoning very hard to follow. Another relevant examlpe of a clear explanation of a similar proof: proof of Lemma 1 in Kohler et al. Notice that they define and explain all the symbols before using them.}

    Now changing integration variable to \(\varepsilon'\) we have \(d\varepsilon = L'p\varepsilon'^{p-1}d\varepsilon'\) and 
    \eq{
        \E_{\xrv}\{ & \rho^2(\xrv_{(1,n)}(\xrv),\xrv)\} \\
        &=\sum_{j=1}^\infty \int_0^\infty\Pr\left\{\rho^2(\xrv_{(1,n)}(\xrv),\xrv) > \varepsilon, {\xrv\in A_j}\right\}d\varepsilon \\
        &\leq \sum_{j=1}^\infty \int_{(-\frac{B}{L'})^{\frac{1}{p}}}^\infty\Pr{\Delta_1^{\xrv} > \varepsilon', {\xrv\in A_j}}L'p\varepsilon'^{p-1}d\varepsilon' \\
        &\leq \sum_{j=1}^\infty \int_{(-B/L')^{1/p}}^\infty \frac{N(\varepsilon')}{en}L'p\varepsilon'^{p-1}d\varepsilon' \\
        &\leq \sum_{j=1}^\infty \int_{(-B/L')^{1/p}}^\infty L'pj^{d-1}\frac{c}{en}\varepsilon'^{p-1-d}d\varepsilon' \\
        &= \sum_{j=1}^\infty \int_0^\infty \frac{c}{en}j^{d-1}L'^{\frac{d}{p}}(\varepsilon-B)^{-\frac{d}{p}}d\varepsilon.
    }

    Since we have segmented the space into a series of sets \(A_j\), we observe that the maximal value the upper bound derived above can take (for each \(j\)) is given by \(\mu(A_j)\). As such, we take the minimum \(\min\left\{\mu(S_{0,j}\backslash S_{0,j-1}),\frac{c}{en}j^{d-1}L'^{\frac{d}{p}}(\varepsilon-B)^{-\frac{d}{p}} \right\}\) from which we can derive a quantity \(\varepsilon_j\) that we can use to split the integral into two computable integrals for each \(j\). \tomcomment{Which integral are you referring to? Every time you refer to a formula, you need to add a number to that formula and refer to it the text.}
    In particular, (defining the shorthand \(\mu_{0,j,j-1}=\mu(S_{0,j}\backslash S_{0,j-1})\)), we know that \(\mu_{0,j,j-1} \geq \frac{c}{en}j^{d-1}L'^{\frac{d}{p}}(\varepsilon-B)^{-\frac{d}{p}}\) which we rearrange to find a lower bound on \(\varepsilon\) for each value of \(j\):
    \eq{
        \varepsilon &\geq B + \left(\frac{c}{en\mu_{0,j,j-1}}j^{d-1}\right)^{p/d}L' := \varepsilon_j.
    }
    Thus, when \(\varepsilon<\varepsilon_j\), \(\min\left\{\mu_{0,j,j-1},\frac{c}{en}j^{d-1}L'^{\frac{d}{p}}(\varepsilon-B)^{-\frac{d}{p}} \right\} = \mu_{0,j,j-1}\) \tomcomment{(bad formatting)} and the reverse when \(\varepsilon\geq\varepsilon_j\).

% An upper bound for the (Euclidean) covering number is, using the argument above:
%     \eq{
%         N(S_{0,j}\backslash S_{0,j-1},\rho_E,(\varepsilon/L)^{1/2p}) &\leq cL^{d/2p}\frac{j^{d-1}}{\varepsilon^{d/2p}}.
%     } 

% Now due to the minimum, the largest \(\varepsilon\) for each \(j\) is given by
% \eq{
%     \varepsilon_j &= \left(\frac{c}{en\mu_{0,j,j-1}}j^{d-1}\right)^{2p/d}
% }

Hence, define \(\mc{E}\) to be
\eq{
    &\sum_{j=1}^\infty \int_0^\infty\min\left\{\mu_{0,j,j-1},\frac{c}{en}j^{d-1}L'^{\frac{d}{p}}(\varepsilon-B)^{-\frac{d}{p}} \right\}d\varepsilon \\
    &\leq \sum_{j=1}^\infty \left(\int_0^{\varepsilon_j}\mu_{0,j,j-1} + \int_{\varepsilon_j}^\infty \frac{c}{en}j^{d-1}L'^{\frac{d}{p}}(\varepsilon-B)^{-\frac{d}{p}}\right)d\varepsilon \\
    &= \sum_{j=1}^\infty\bigg[(\varepsilon_j-B)\mu_{0,j,j-1} + B\mu_{0,j,j-1} \\
    &\qquad + \frac{p}{d-p}\frac{c}{en}j^{d-1}L'^{\frac{d}{p}}(\varepsilon-B)^\frac{p-d}{p}\bigg] \\
    &= \sum_{j=1}^\infty(\varepsilon_j-B)\bigg[\mu_{0,j,j-1} \\
    &\qquad +\frac{p}{d-p}\frac{c}{en}j^{d-1}\left(\frac{c}{en\mu_{0,j,j-1}}\right)^{-1}j^{1-d}\bigg] +B\\
    &= \sum_{j=1}^\infty\frac{d}{d-p}\mu_{0,j,j-1}L'\left(\frac{c}{en\mu_{0,j,j-1}}j^{d-1}\right)^{p/d} + B\\
    &= c'\sum_{j=1}^\infty\mu_{0,j,j-1}^\frac{d-p}{d}j^\frac{p(d-1)}{d}n^{-\frac{p}{d}} + B
}
where we note that \(\frac{p-d}{p}<0\) is necessary for the upper limit of the second integral to vanish and that the sum over the terms \(\mu_{0,j,j-1}\) sums to unity.

Finally we apply H\"{o}lder's inequality with \(p'=d/p,\, q'=\frac{d}{d-p}\). Let \(a+b=\frac{p(d-1)}{d}\) and \(\alpha=a\cdot p'\) and \(\beta=b\cdot q'\) and set 
\eq{
    \mc{E} &\leq B + c'n^{-\frac{p}{d}}\left(\sum_{j=1}^\infty j^\alpha\right)^\frac{p}{d}\left(\sum_{j=1}^\infty j^\beta \mu_{0,j,j-1}\right)^\frac{d-p}{d}
}
then we know that \(\alpha < -1\) in order for the first sum to converge. Additionally, \(a=\alpha\cdot\frac{p}{d}\) and \(b=\beta\cdot\frac{d-p}{d}\). We can combine these constraints to see that 
\eq{
    \alpha p + \beta(d-p) &= p(d-1) \\
    \beta &= \frac{p(d-1)-\alpha p}{d-p} > \frac{p(d-1)+p}{d-p} \\
    &= \frac{pd}{d-p}
}
which provides our other requirement for convergence of the second sum, which represents \(\E\norm{\xrv}^\beta\) and converges due to \cref{lem:finite_jsum}.

We then define a new constant \(c''\) that absorbs the convergent sums to say that
\eq{
    \mc{E} &\leq B + c''n^{-\frac{p}{d}}.
}

% In what follows, set \(c_1=cL^{d/2p}\)
% \eq{
%     \mc{E} & = \sum_{j=1}^\infty \int_0^\infty\min\left\{\mu(S_{0,j}\backslash S_{0,j-1}), \frac{1}{en}N(S_{0,j}\backslash S_{0,j-1},\norm{\cdot},(\varepsilon/L)^{1/2p})\right\}d\varepsilon \\
%     &\leq \sum_{j=1}^\infty\left(\int_0^{\varepsilon_j}\mu_{0,j,j-1} + \int_{\varepsilon_j}^\infty \frac{c_1}{en}\frac{j^{d-1}}{\varepsilon^{d/2p}}\right)d\varepsilon \\
%     &= \sum_{j=1}^\infty\left[\mu_{0,j,j-1}\varepsilon_j + \frac{2p}{d-2p}\frac{c_1}{en}j^{d-1}\left(\frac{c_1}{en}j^{d-1}\right)^\frac{2p-d}{d}\mu_{0,j,j-1}^\frac{d-2p}{d}\right] \\
%     &= \left(\frac{c_1}{en}\right)^{2p/d}\sum_{j=1}^\infty j^\frac{2pd-2p}{d}\left(\mu_{0,j,j-1}^\frac{d-2p}{d} + \frac{2p}{d-2p}\mu_{0,j,j-1}^\frac{d-2p}{d}\right) \\
%     &= c' L n^{-\frac{2p}{d}}\sum_{j=1}^\infty j^\frac{2pd-2p}{d}\mu_{0,j,j-1}^\frac{d-2p}{d}
% }
% noting that \(\frac{2p-d}{d} < 0\) so the upper limit of the second integral vanishes and defining a new constant \(c'\) to absorb the other constants.

% Finally, applying Hölder's inequality, with \(p'=d/2p,q'=\frac{d}{d-2p}\) we have
% \eq{
%     \mc{E} &\leq c''Ln^{-\frac{2p}{d}}\left(\sum_{j=1}^\infty j^\alpha\right)^\frac{2}{d}\left(\sum_{j=1}^\infty j^\beta\mu_{0,j,j-1}\right)^\frac{d-2p}{d} \\
%     &\leq c'''n^{-\frac{2p}{d}}
% }
% provided \(\alpha < -1\) so that the first sum converges and \(\beta > \frac{2pd}{d-2p}\).
% \(\frac{2pd-2p}{d}=a+b, \, \alpha = a\cdot p'< -1, \, b > \frac{2pd-2p}{d} +\frac{2p}{d} = 2, \, \beta = b\cdot q' > \frac{2pd}{d-2p}\). Additionally, the second sum represents \(\E\norm{\xrv}^\beta\) and hence converges due to \cref{lem:finite_jsum}.
  
Finally we put these pieces together. We divide the full dataset into \(m+1\) segments such that the first \(m\) have length \(\floor*{\frac{n}{m}}\) and \(\tilde{\xrv}_j^{\xv}\) is the nearest-neighbour to \(\xv\) from the \(j^{th}\) segment:

% \robertcomment{********* Unless I've misunderstood there might be a problem below: To get the penultimate inequality you have conditioned on the nearest amongst the whole $n$ being within $\Delta$ of $\bm{x}$ whereas obtaining the upper bound in the inequality seems to require the stronger condition that be within $\Delta$ for the nearest neighbour amongst only $\floor{\frac{n}{m}}$ (rather than all $n$) points. Also it requires that stronger condition to hold simultaneously for all of the $m$ segments }
% \antcomment{I think you are correct. The conditioning, at least for Matern/SE kernels holds for all \(\Delta>0\) so isn't so strong a statement. For kernels requiring a Taylor expansion to work, maybe a stronger conditioning set is required?}
Finally we put these pieces together. We divide the full dataset into \(m+1\) segments such that the first \(m\) have length \(\floor*{\frac{n}{m}}\) and \(\tilde{\xrv}_j^{\xv}\) is the nearest-neighbour to \(\xv\) from the \(j^{th}\) segment:

\eq{
    \Ex{\avg{\eps_i}} &= \frac{1}{m}\sum_{i=1}^m\Ex{\rho^2(\xrv_{(i)}(\xrv),\xrv)} \\
    &\leq \frac{1}{m}\sum_{j=1}^m\Ex{\rho^2(\tilde{\xrv}_j^{\xrv},\xrv)} \\
    &= \Ex{\rho^2(\tilde{\xrv}^{\xrv}_1,\xrv)} \\
    &= \Ex{\rho^2(\xrv_{(1,\floor*{\frac{n}{m}})}(\xrv),\xrv)} \\
    &\leq c''L'\floor*{\frac{n}{m}}^{-p/d} \\
    &\leq C\left(\frac{n}{m}\right)^{-p/d}
}
\hfill\(\square\)



Here we give a technical condition to ensure that the sums over \(j\) in the above proofs converge (used directly in \cref{lem:eps_i}).
\begin{lemma}[Technical condition for unbounded input]
    \label{lem:finite_jsum}
    Assume that \(\E\norm{\xrv}^\beta<\infty\) and adopting all of the prior notation, then it can be shown that
    \[\sum_{j=1}^\infty j^\beta \mu(S_{0,j}\backslash S_{0,j-1}) < \infty.\]
\end{lemma}
\begin{proof}
Suppose \(\mc{X}=\bigcup_{j=1}^\infty A_j\) with \(A_i\cap A_j = \emptyset\) if \(i\neq j\), then (setting \(A_j=S_{0,j}\backslash S_{0,j-1}\))
\eq{
    \E\norm{\xrv}^\beta &= \int_0^\infty \Pr(\norm{\xrv}^\beta > \varepsilon)d\varepsilon \\
    &= \int_0^\infty \sum_{j=1}^\infty \Pr(\norm{\xrv}^\beta > \varepsilon, X \in A_j)d\varepsilon \\
    &= \sum_{j=1}^\infty \int_0^\infty \int_{A_j}\Pr(\norm{\xrv} > \varepsilon^{1/\beta})\mu(d\xv)d\varepsilon \\
    &=\sum_{j=1}^\infty \int_0^{j^\beta}\int_{A_j}(1-\mu(S_{0,\varepsilon^{1/\beta}}))\mu(d\xv)d\varepsilon \\
    &\leq \sum_{j=1}^\infty \int_0^{j^\beta}\mu(A_j)d\varepsilon \\
    &= \sum_{j=1}^\infty j^\beta \mu(A_j)
}
which gives us an upper bound.

Note that \(\E\norm{\xrv}\geq\E\floor{\norm{\xrv}}=\sum_{n=1}^\infty \Pr(\norm{\xrv}\geq n)\) 
% and \(\Pr(\floor{\norm{\xrv}}\geq j\given X\in A_j)=1\) a.s., 
\eq{
    \E\norm{\xrv}^\beta &= \sum_{j=1}^\infty \E[\norm{\xrv}^\beta\given A_j]\mu(A_j) \\
    &\geq \sum_{j=1}^\infty (j-1)^\beta \Pr(\floor{\norm{\xrv}}\geq j-1\given A_j)\mu(A_j) \\
    &= \sum_{j=1}^\infty (j-1)^\beta \mu(A_j)
}
using Markov's inequality to say \(\E[\norm{\xrv}^\beta\given  A_j] \geq j^\beta \Pr(\norm{\xrv}\geq j \given A_j)\) and that for \(\xrv \in A_j\), \(\floor{\norm{\xrv}}=j-1\).

% Now if this is true, then \(j^{\beta-1}\leq\E\norm{\xrv}^{\beta-1}\given A_{j+1} \leq \E\norm{\xrv}^\beta\given A_{j+1}\) which gives
% \eq{
%     \E\norm{\xrv}^\beta\given A_j &\geq j^\beta - \beta j^{\beta-1} \geq j^\beta - \beta\E\norm{\xrv}^\beta \given A_{j+1}
% }
% which we rearrange, and thus
% \eq{
%     \E\norm{\xrv}^\beta &\geq \sum_{j=1}^\infty \left[j^\beta - \beta\E\norm{\xrv}^\beta\given A_j\right]\mu(A_j) \\
%     &\geq \frac{1}{1+\beta}\sum_{j=1}^\infty j^\beta\mu(A_j).
% }
Combining these gives
\eq{
    \sum_{j=1}^\infty(j-1)^\beta\mu(A_j) &\leq \E\norm{\xrv}^\beta \leq \sum_{j=1}^\infty j^\beta\mu(A_j)
}

Using this result and that \((j-1)^\beta \geq j^\beta - \beta j^{\beta-1}\) we can say
\eq{
    \sum_{j=1}^\infty j^\beta \mu(A_j) &\leq \sum_{j=1}^\infty(j-1)^\beta\mu(A_j) + \beta \sum_{j=1}^\infty j^{\beta-1}\mu(A_j) \\
    &\leq \E\norm{\xrv}^\beta + \beta\E\norm{\xrv}^{\beta-1} \\
    &< \infty
}
since \(\E\norm{\xrv}^\beta<\infty \implies \E\norm{\xrv}^{\beta-1}<\infty.\)
\end{proof}
